# Supplementary material for: Flexible and scalable privacy assessment for very large datasets, with an application to official governmental microdata
Source: arXiv:2204.13734 source file (2022-07-25)
Supplement: Supplementary file 1 [file appendix-anon-experiments.tex]

Syntactic or deterministic methods apply syntactic restrictions on their outputs to avoid the unintended disclosure of information. Among the restrictions usually applied we have \qm{generalization}, \qm{suppression}, and \qm{swapping}.
\begin{itemize}
	\item \textbf{Generalization}: values of an attribute are replaced by a more generic category, e.g. age ranges instead of exact values.
	
	\item \textbf{Suppression}: values of an attribute are replaced by a special value, e.g. hiding of some final numbers of the ZIP code by using an asterisk.
	
	\item \textbf{Swapping}: values of an attribute for different records are swapped. Differently from generalization and suppression, which are non-perturbative techniques, swapping can be seen as a perturbative technique since it may introduce untrue information to the released data.
\end{itemize}

Samarati and Sweeney, observing that just a few quasi-identifying attributes were enough to enable the re-identification of individuals in de-identified data, proposed in 1998 a novel anonymization method called \emph{k}-\emph{anonymity} \cite{Samarati98}. Given a dataset, it is considered to be \emph{k}-anonymous if any attempt to link quasi-identifying attributes to sensitive information creates a many-to-one mapping in which at least \emph{k} records map to the same sensitive information, i.e. the dataset would be partitioned in blocks of at least \emph{k} records in each. In order to achieve this result, Samarati and Sweeney proposed the use of generalization and suppression.

%However, as shown by Aggarwal \cite{Aggarwal05} in 2005, \emph{k}-anonymity robustness is inversely dependent on the dimensionality of the dataset, i.e. on the number of attributes that can be used as quasi-identifiers. Furthermore, Machanavajjhala et al. unveiled in 2007 two severe weaknesses in \emph{k}-anonymity \cite{Machanavajjhala07}. First, they showed that a low diversity in the values assumed by a sensitive attribute allows an attacker to discover those values within a block of records. Second, \emph{k}-anonymity does not provide any privacy guarantee against the use of background knowledge by an adversary, i.e. the use of auxiliary information.

%In that same paper describing \emph{k}-anonymity's weaknesses, Machanavajjhala et al. proposed an alternative approach called \emph{l}-\emph{diversity}, which improves on \emph{k}-anonymity by also requiring at least \emph{l} \qm{well-represented} values for the sensitive attribute within each block. By \qm{well-represented} values, they suggested some different interpretations, the most common being \emph{distinct} \emph{l}-\emph{diversity}, which requires at least \emph{l} distinct values for the sensitive attribute within each block, automatically satisfying \emph{k}-anonymity with \emph{k} equal to \emph{l}. This interpretation does not prevent probabilistic inference attacks, though, since it does not prevent a value from appearing much more frequently in a block of records than other values, which increases the likelihood of that value for any individual who may hold a record withing the given block.

Another anonymization method was proposed by Machanavajjhala et al. in 2007, called \emph{l}-\emph{diversity} \cite{Machanavajjhala07}, which requires at least \emph{l} \qm{well-represented} values for the sensitive attribute within each block. By \qm{well-represented} values, they suggested some different interpretations, including \emph{entropy} \emph{l}-\emph{diversity} and \emph{recursive} (\emph{c,l})-\emph{diversity}.

A table is \emph{entropy} \emph{l}-\emph{diverse} if for every generalized block $q^*$ of records
\begin{align}
	- \sum_{s \in S} p_{(q^*,s)} \log(p_{(q^*,s')}) \geq \log(l),
\end{align}
where $p_{(q^*,s)} = \frac{n_{(q^*,s)}}{\sum_{s' \in S} n_{(q^*,s')}}$ is the fraction of tuples in the generalized block with sensitive attribute value equal to $s$. Hence, every generalized block has at least \emph{l} distinct values for the sensitive attribute.

Now consider a generalized block $q^*$ of records and let $r_i$ denote the number of times the $i^{th}$ most frequent sensitive value among the $m$ possible values appears in that block. Given an arbitrary constant $c$, a table is \emph{recursive} (\emph{c,l})-\emph{diversity} if every generalized block satisfies $r_1 < c(r_l + r_{l+1} + \cdots + r_m)$.

In the same year, Li et al. proposed another approach to anonymization called \emph{t}-\emph{closeness} \cite{Li07}. Differently from other syntactic methods, \emph{t}-\emph{closeness} also has some characteristics found in semantic methods. Because it tries to limit how much information an adversary can gather from the published dataset, it applies the \qm{uninformative principle}.~\footnote{The uninformative principle holds if the adversary's \emph{a posteriori} knowledge on any data holder is not much larger than their \emph{a priori} knowledge.}

The \emph{t}-\emph{closeness} Principle states that an equivalence class is said to have \emph{t}-\emph{closeness} if the distance between the distribution of a sensitive attribute in this class and the distribution of the attribute in the whole table is no more than a threshold \emph{t}. A table is said to have \emph{t}-\emph{closeness} if all equivalence classes also have it.~\footnote{In their original work, Li et al. used the \emph{Earth Mover Distance} measure as their \emph{t}-\emph{closeness} requirement.}

For our experiments, we have used the ARX software with our proposed update that allows it to work with larger datasets in order to anonymize the dataset for the School Census of 2018. We have tried to use all the three main syntactic methods described above, namely \emph{k}-\emph{anonymity}, \emph{l}-\emph{diversity}, and \emph{t}-\emph{closeness}.

For \emph{k}-\emph{anonymity}, we have successfully created six versions of the dataset, each using one value for the parameter \emph{k}: 4, 8, 12, 16, 20, and 24.

For \emph{l}-\emph{diversity}, we have tried to use both \emph{entropy} \emph{l}-\emph{diversity} and \emph{recursive} (\emph{c,l})-\emph{diversity} for values of \emph{l} around 2 and for values of \emph{c} around 40 for the disability sensitive attribute, considering the skewness of this attribute. However, the only solution found would cause the complete suppression of the considered quasi-identifying attributes.

For \emph{t}-\emph{closeness}, we have successfully created five versions of the dataset, each using one value for the parameter \emph{t}: 0.1, 0.2, 0.3, 0.4, and 0.5. For every version, we have considered the disability attribute as the sensitive one.

Given the anonymized datasets, we have performed both re-identification and attribute-inference attacks, for both deterministic and probabilistic measurements of success. For the attribute-inference attacks, we have considered the disability attribute as the sensitive one. Table~\ref{tab:anonymization} summarizes our results, also presented in Figure~\ref{fig:anonymization}.

\begin{figure*}[tb]
	\centering
	\begin{subfigure}[t]{0.48\linewidth}
		\centering
		\includegraphics[width=\linewidth]{figures/leakages-k-anonymity-2018}
		\caption{}
		\label{fig:k-anonymous}
	\end{subfigure}
	\begin{subfigure}[t]{0.48\linewidth}
		\centering
		\includegraphics[width=\linewidth]{figures/leakages-t-closeness-2018}
		\caption{}
		\label{fig:t-closed}
	\end{subfigure}
	\caption{Changes in deterministic and probabilistic leakages for re-identification and attribute-inference according to the applied anonymization technique: \emph{k}-\emph{anonymity} and \emph{t}-\emph{closeness}. For the attribute-inference attacks, we have considered the disability attribute as the sensitive one.}
	\label{fig:anonymization}
\end{figure*}

\begin{table*}[tb]
	\centering
	
	\begin{small}
		$
		\begin{array}{|>{\centering\arraybackslash\small}m{0.1\linewidth}|>{\centering\arraybackslash\small}m{0.18\linewidth}|>{\centering\arraybackslash\small}m{0.18\linewidth}|>{\centering\arraybackslash\small}m{0.18\linewidth}|>{\centering\arraybackslash\small}m{0.18\linewidth}|}
			\cline{2-5}
			\multicolumn{1}{c|}{}
			& \multicolumn{2}{>{\centering\arraybackslash\small}m{0.36 \linewidth}|}{\textbf{Re-identification}}
			& \multicolumn{2}{>{\centering\arraybackslash\small}m{0.36 \linewidth}|}{\textbf{Attribute-inference}} \\
			\hline
			\textbf{Dataset}
			& \textbf{Deterministic} & \textbf{Probabilistic}
			& \textbf{Deterministic} & \textbf{Probabilistic} \\
			\hline
			Original & 0.96342560 & 0.98138799 & 0.99890918 & 1.02450214 \\
			\hline
			$k=4$ & 0.00000000 & 0.00008369 & 0.00048254 & 1.00000000 \\
			\hline
			$k=8$ & 0.00000000 & 0.00006974 & 0.00039663 & 1.00000000 \\
			\hline
			$k=12$ & 0.00000000 & 0.00029857 & 0.00079773 & 1.00000000 \\
			\hline
			$k=16$ & 0.00000000 & 0.00002790 & 0.00008977 & 1.00000000 \\
			\hline
			$k=20$ & 0.00000000 & 0.00002790 & 0.00008977 & 1.00000000 \\
			\hline
			$k=24$ & 0.00000000 & 0.00002790 & 0.00008977 & 1.00000000 \\
			\hline
			$t=0.1$ & 0.00000000 & 0.00002790 & 0.00008977 & 1.00000000 \\
			\hline
			$t=0.2$ & 0.00000000 & 0.00008369 & 0.00048254 & 1.00000000 \\
			\hline
			$t=0.3$ & 0.00000023 & 0.00002750 & 0.00013258 & 1.00000000 \\
			\hline
			$t=0.4$ & 0.00000073 & 0.00005467 & 0.00026102 & 1.00000000 \\
			\hline
			$t=0.5$ & 0.00000166 & 0.00006615 & 0.00041118 & 1.00000000 \\
			\hline
		\end{array}
		$
	\end{small}
	\caption{Changes in deterministic and probabilistic leakages for re-identification and attribute-inference according to the applied anonymization technique: \emph{k}-\emph{anonymity} and \emph{t}-\emph{closeness}. For the attribute-inference attacks, we have considered the disability attribute as the sensitive one.}
	\label{tab:anonymization}
\end{table*}
